# Supplementary material for: Revisiting the stable structure of the Cu$_{4}$ complex in silicon
Source: arXiv:1912.11586 ancillary file (2020-05-14)
Supplement: Supplementary file 1 [file supplement.pdf]

# Supplemental materials

Takayoshi Fujimura and Koun Shirai

*Nanoscience and Nanotechnology Center,*

*The Institute of Scientific and Industrial Research (ISIR),*

*Osaka University, 8-1 Mihogaoka, Ibaraki, Osaka 567-0047, Japan*

(Dated: March 25, 2020)

## Abstract

This part provides auxiliary materials for the main article "Revisiting the stable structure of $Cu_4$ complex in silicon"

PACS numbers:

## S1. Supercell size dependence

In the main paper, calculations are performed on supercells of size $2\times2\times2$ of conventional unit cells. To ensure the accuracy of the calculations, how the size of supercell influences the formation energy has been performed by extending the size of supercells. The calculations in this section were performed by a different code PHASE[1] based on the same principles as in the main paper, owing to a technical reason. The ingredients of PHASE code are thus plane-wave expansion and pseudopotentials. Here, the Perdew-Burke-Ernzerhof type (GGA-PBE)[2] was used for the electron-correlation functional and ultrasoft pseudopotentials of Vanderbilt type[3] were used. The cutoff energies of 25 and 225 Ry for plane-wave expansion and charge density, respectively. Atomic positions are optimized until all the forces acting on atoms are less than $1 \times 10^{-3}$ Hatree/Bohr. The used supercells are cubes of the unit cell size $a_s$: $a_s$ =2, 3, and 4 in the unit $a_0$ (the lattice parameter of silicon).

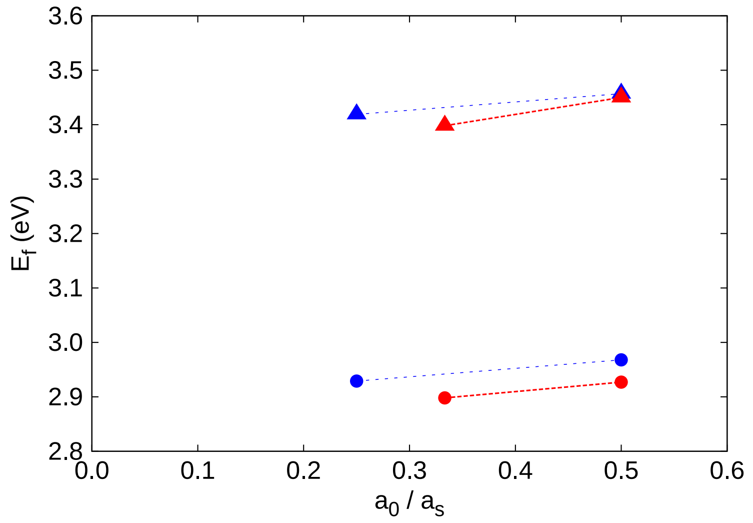


FIG. 1: The dependence of the formation energy $E_f$ of $Cu_4$ on the size of supercells. Triangles indicate $C$-type and circles indicate $T$-type $Cu_4$. Equivalent **k**-meshes are connected by colors: blue symbols indicate a $2^3$-mesh for the supercell of $a_s = 2a_0$ and $\Gamma$ point for the supercell of $a_s = 4a_0$; red symbols indicate a $3^3$-mesh for the supercell of $a_s = 2a_0$ and a $2^3$-mesh for the supercell of $a_s = 3a_0$.

Figure 1 shows the formation energy $E_f$ of $C$- and $T$-types of $Cu_4$ complexes versus the size of supercells. The change of $E_f$ with $a_s$ is only 0.04 eV up to $a_s = 4$ for both $C$-

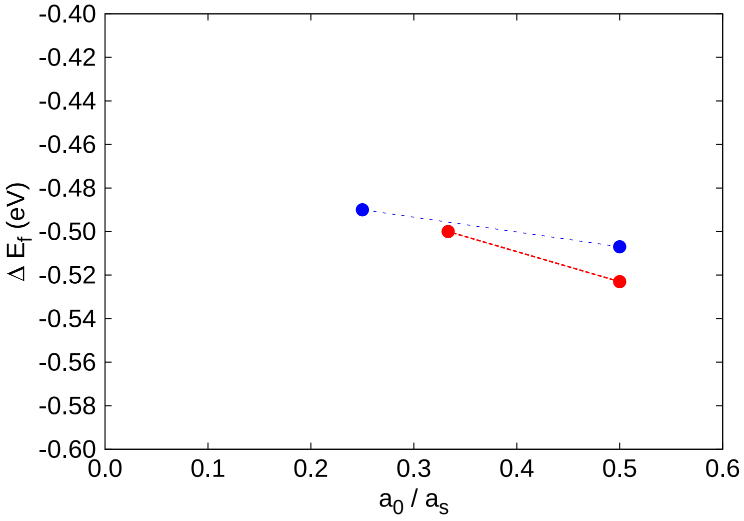


FIG. 2: Difference in the formation energy $\Delta E_f = E_f[T] - E_f[C]$ versus $a_0/a_s$. The colors are used in the same meaning as in Fig. 1.

and $T$-types. The difference in the formation energy $\Delta E_f = E_f[T] - E_f[C]$ with $a_s$ is well converged within 0.03 eV, as shown in Fig. 2. Variations in this order have no consequence on the present study. Therefore, the calculations of the main text have sufficient accuracy for discussing the stability of the $Cu_4$ complexes. This is true also for the $k$ mesh. The result of use of the $2^3$ mesh is well converged.

## S2. Other complexes of $M_4$-type

Other complexes of $M_4$-type, where $M$ =H, Li, Br, have been studied to investigate the chemical trends in $M_4$ complexes. Table I summarizes the structural characteristics of $M_4$ complexes, together with the difference in the formation energy $\Delta E_f = E_f[T] - E_f[C]$. In all the cases, $C$-type, $M_{(s)}M_{3(i)}$, is not stable. For Li, $C$-type is only metastable, while for H and Br it is unstable; the later two complexes of $C$-type spontaneously collapse to different structures. The structures of stable states are listed in Table I. For the reference bond, the "natural" bond length $M - M$ is listed. Here, the natural bond length is meant as the distance between the nearest neighboring atoms in the metallic phase for Li and Cu, and as the bond length of the diatomic molecules for Br and H. Among them, only Cu has

TABLE I: Structures of $M_4$ complexes in silicon and the difference in the formation energy $\Delta E_f = E_f[T] - E_f[C]$ between $C$- and $T$-types. In the column $\Delta E_f$, the notation $-$ indicates that $C$ type is unstable. In the column of bond length, 3×2.40, for example, should be read as three bonds with the length 2.40 Å. For the meaning of natural length, refer to the text.

| Complex | $\Delta E_f$ | Bond length (Å) | | | Description |
|---|---|---|---|---|---|
| | (eV) | $M$−Si | $M-M$ | Natural | |
| $H_4$ | – | 1.50 | 3×1.70 | 0.71 | Double-layered tetrahedra |
| $Li_4$ | -0.34 | 3×2.40 | 3×2.57 | 3.04 | Dodecahedron |
| $Cu_4$ | -0.28 | 3×2.44 | 3×2.54 | 2.55 | Dodecahedron |
| $Br_4$ | – | 2.32 | 2×2.82, 3.07 | 2.28 | Dodecahedron with large distortion |

approximately the same length as the natural bond length. The structure of $Br_4$ is far from the regular tetrahedron. From these comparisons, it is found that the $Cu_4$ tetrahedron has a special role of forming the molecular unit, in addition to the role of electron dopant. It behaves as molecular unit which itself has stability.

## S3. Wavefunctions of the gap states of the $Cu_4$ tetrahedron

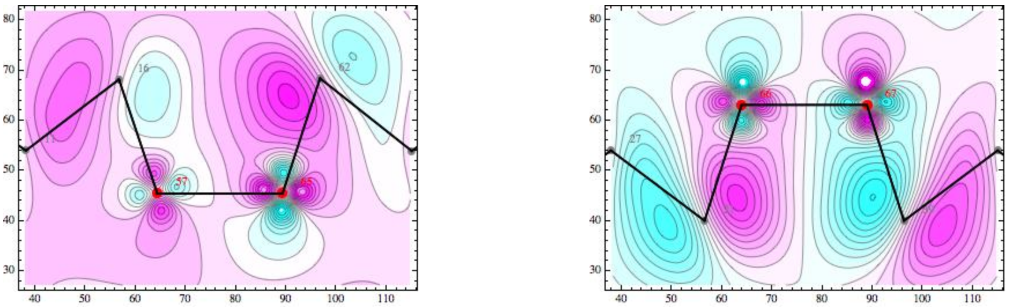

FIG. 3: Wavefunction of 146th band (imaginary part).

The bonding nature of the $T$-type $Cu_4$ tetrahedron is analyzed by calculating wavefunctions. The wavefunctions $\Psi_k$ of the gap states at $\Gamma$ point are shown in Figs. 3, 4, and 5. In the present supercell model, three states from 146 to 148th bands from the lowest band are the gap states. The cut plane is the same as that of Fig. 4 of the main paper. Red and blue lines indicate the different signs of wavefunctions. Note that the scales of wavefunctions

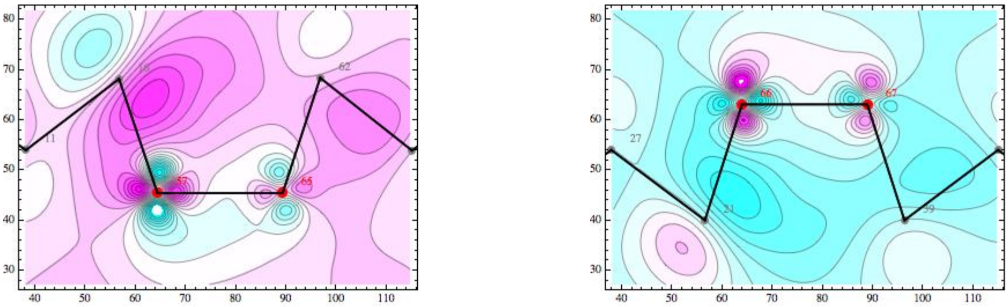

FIG. 4: Wavefunction of 147th band (real part).

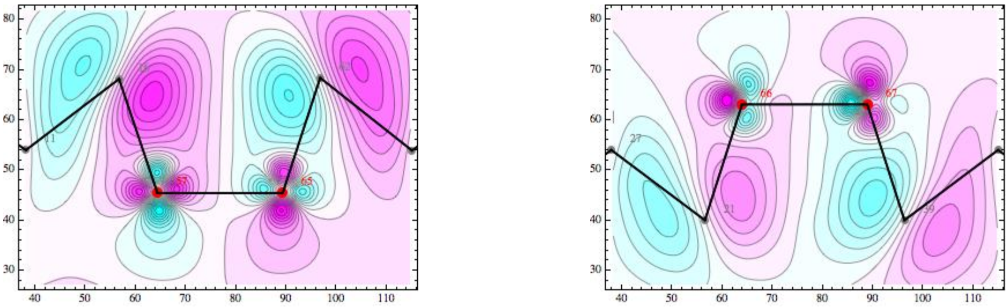

FIG. 5: Wavefunction of 148th band (real part).

are not the same among different plots. The atom labels are the same as these given in Fig. 1 of the main paper. In all the cases, it is observed that the band has a character of $d\gamma$ orbitals oriented in the $z$-axis (the upward direction in the figure), and that the $d\gamma$ orbitals are coupled with $p$ orbitals of Si in the antibonding manner. The antibonding character is seen in the appearance of a node in the line of the Cu$-$Si bond.

## S4. Molecular orbitals of the $Cu_4$ tetrahedron

A molecular-orbital description for the $Cu_4$ tetrahedron in silicon is given. The $Cu_4$ tetrahedron has 44 valence electrons. $T$-type $Cu_4$ tetrahedron replaces a Si atom—removing a Si atom alone creates four dangling bonds. Out of the 44 electrons, four electrons fill four half-filled dangling bonds. The remaining 40 electrons are available to form the molecular orbitals of the $Cu_4$ tetrahedron. In the $Cu_4$, each atom supplies five $d$ orbitals with the total number of $d$ orbitals being 20. These orbitals are symmetrized to 8 orbitals, as $a_1 + 2e + 2t_1 + 3t_2$. The explicit expressions of the symmetrized wavefunctions are given in Table II, where $n$th orbital of $j$th symmetry is denoted as $\phi_{jn}$.

TABLE II: Symmetrized wavefunctions $\phi_{jn}$ of the $Cu_4Si_4$ dodecahedron, where $j$ is the index of symmetry and $n$ is an additional index within $j$th symmetry. $\phi_{jn}$ is given by a linear combination of atomic $d$ orbitals $\chi_m^i$ at $i$-th site. In the Table, the coefficients for $\chi_m^i$ are listed in a manner $(\chi_m^1; \chi_m^2; \chi_m^3; \chi_m^4)$, where $m$ denotes the component of a set of functions, either $\vec{d\gamma}$ or $\vec{d\varepsilon}$. The normalization factors are omitted. Minus sign is expressed by bar. For $\phi_{jn}$ of multi-dimensional representations, only one component, which is transformed as either $x^2 - y^2$ or $z$, is shown.

| $j$ | $n$ | Symmetrized vectors |
|---|---|---|
| | | $\vec{d\gamma} = (3z^2 - r^2, x^2 - y^2)$ |
| $e$ | 1 | (0,1; 0,1; 0,1; 0,1) |
| $t_1$ | 1 | $(0,1;\ 0,1;\ 0,\bar{1};\ 0,\bar{1})$ |
| $t_2$ | 2 | $(1,0;\ 1,0;\ \bar{1},0;\ \bar{1},0)$ |
| | | $\vec{d\varepsilon} = (yz, zx, xy)$ |
| $a_1$ | 1 | $(1,1,1;\ \bar{1},\bar{1},1;\ 1,\bar{1},\bar{1};\ \bar{1},1,\bar{1})$ |
| $e$ | 2 | $(\bar{1},1,0;\ 1,\bar{1},0;\ 1,1,0;\ \bar{1},\bar{1},0)$ |
| $t_1$ | 2 | $(1,\bar{1},0;\ \bar{1},1,0;\ 1,1,0;\ \bar{1},\bar{1},0)$ |
| $t_2$ | 3 | $(0,0,1;\ 0,0,1;\ 0,0,\bar{1};\ 0,0,\bar{1})$ |
| | 4 | $(1,1,0;\ \bar{1},\bar{1},0;\ \bar{1},1,0;\ 1,\bar{1},0)$ |

The Hamiltonian matrix is constructed by the tight-binding approximation. Matrix elements of Slater–Koster type are used.[?] The explicit forms of the symmetrized Hamiltonian matrices $H$ are given in Table III. Let us consider coupling of the molecular orbitals of the $Cu_4$ tetrahedron to the host bands. We use a crude approximation that the valence bands of the host is represented only by triply degenerated $\Gamma_{25'}$ bands at $\Gamma$ point, because we are here interested only in the mechanism of the creation of the gap state. Since only $t_2$ symmetry is compatible with $\Gamma_{25'}$, only the $H(t_2)$ block is relevant for investigation of the gap states. The host $\Gamma_{25'}$ band is created by a linear combination of $sp^3$ hybrid orbitals from Si atoms of the $Cu_4Si_4$ dodecahedron. In the tight-band approximation, four hybrid orbitals pointing to the center of the $Cu_4$ tetrahedron are used. One of these hybrid orbital $\phi_{t_2,1}$ appears at the first element of a $4 \times 4$ matrix $H(t_2)$. Also, an approximation was made that the four Si atoms are slightly displaced inward so as to deform the dodecahedron to a cube. On this approximation, all Si and Cu atoms are placed on the corners of the cube in Fig. 1 of

the main paper, and accordingly many angles become exactly the right angle. This makes the form of matrix elements simpler. Only at the last stage of numeric calculation, the real values of the bond lengths were used.

TABLE III: Hamiltonian matrices decomposed by symmetrized wavefunctions. The order of the symmetrized wavefunctions is in accordance with the index $n$ of Table II. For the sake of simplicity, only upper-right elements are shown.

$$H(e) = \begin{pmatrix} \frac{1}{8}\left(3V_{dd\sigma} + 12V_{dd\pi} + 9V_{dd\delta}\right), & \frac{3}{4\sqrt{2}}\left(V_{dd\sigma} + V_{dd\delta}\right) \\ \cdot & \frac{1}{4}\left(-3V_{dd\sigma} - 2V_{dd\pi} + V_{dd\delta}\right) \end{pmatrix},$$

$$H(t_1) = \begin{pmatrix} \frac{1}{8}\left(-3V_{dd\sigma} + 4V_{dd\pi} - 9V_{dd\delta}\right), & \frac{9}{16}V_{dd\delta} \\ \cdot & \frac{1}{4}\left(3V_{dd\sigma} - 2V_{dd\pi} + 5V_{dd\delta}\right) \end{pmatrix},$$

$$H(t_2) = \begin{pmatrix} 0, & -\frac{2}{\sqrt{3}}V_{pd\sigma}, & -\frac{2}{\sqrt{3}}V_{pd\pi}, & -\frac{4}{\sqrt{6}}V_{pd\pi} \\ \cdot & \frac{1}{8}\left(V_{dd\sigma} - 12V_{dd\pi} + 3V_{dd\delta}\right), & \frac{\sqrt{3}}{4}\left(-V_{dd\sigma} + V_{dd\delta}\right), & \frac{1}{4}\sqrt{\frac{3}{2}}\left(-V_{dd\sigma} + V_{dd\delta}\right) \\ \cdot & \cdot & \frac{1}{8}\left(3V_{dd\sigma} - 4V_{dd\pi} - 3V_{dd\delta}\right), & \frac{1}{\sqrt{2}}\left(V_{dd\pi} - V_{dd\delta}\right) \\ \cdot & \cdot & \cdot & \frac{1}{16}\left(3V_{dd\sigma} - 3V_{dd\pi} - V_{dd\delta}\right) \end{pmatrix},$$

Handy formulae for the matrix elements are given by Harrison.[?] The values have been well tested for Si. For Cu, the values is more affected by the local environment, namely, the effect of the electron shielding. We only hope that this treatment is not too bad. By using numerical values in Solid State Table in Ref. **?** , we obtained an energy spectrum of Fig. 9. Here, for the difference of atomic energies $\varepsilon_d - \varepsilon_p$, a value of 1 eV different from the listed value in Ref. **?** was used; otherwise the same values are used.

The highest band of $t_2$ symmetry can be regarded as the gap state $\Psi_{\Gamma_{25'}}$ of the crystal, for both point defect $Cu_{(s)}$ and the $Cu_4$ complex, because this state is only the antibonding state in the present subspace spanned by the $p$ orbitals of Si and the $d$ orbitals of Cu. There is, however, a difference in the orbital character between the point defect $Cu_{(s)}$ and the $Cu_4$ complex. The $t_2$ band of $Cu_4$ is mainly composed of the $d\gamma$ orbitals of Cu atoms, whereas that of the point defect $Cu_{(s)}$ is composed of the $d\varepsilon$ orbitals of the $Cu_{(s)}$ atom. By inspecting

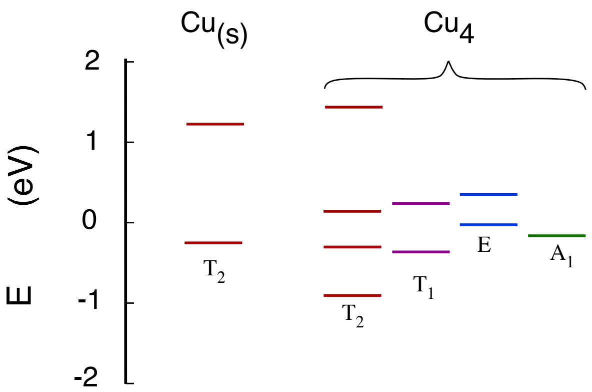


FIG. 6: Energy levels of $T$-type $Cu_4$, compared with that of $Cu_{(s)}$.

the explicit form of $H(t_2)$, we can understand the reason. For the $Cu_4$ case, the host $\Gamma_{25'}$ band is composed of the $d\gamma$-component with a strong $pd\sigma$ bond, while it is composed of the $d\varepsilon$-component with a relatively weak $pd\pi$ bond. On the other hand, for the case of point defect $Cu_{(s)}$, $\Gamma_{25'}$ band is composed of $d\varepsilon$ orbitals only.

## S5. DOS of $M_4$ complexes

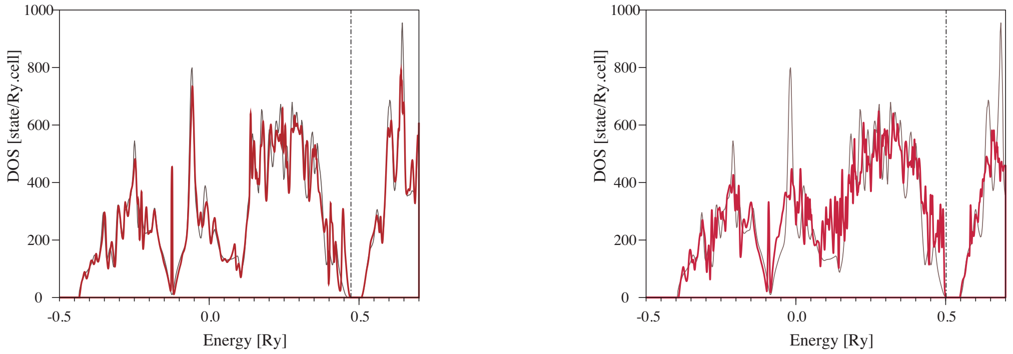


FIG. 7: DOS of $Li_4$ and $Br_4$ complexes (red line). DOS of bulk Si is shown by a black line. The top of occupied bands is indicated by a dashed line.

The DOS of $M_4$ complexes are shown in Figs. 7 and 8. It is observed that, in all the cases, the band gap is almost not affected by doping. However, for $Li_4$ and $Br_4$, a peak is observed at the top of valence band, and for $Li_4$ the tail of the peak is slightly extended to the band gap. For the $Li_4$ case, the peak portion is a localized state of $Li_4$ and may correspond to the

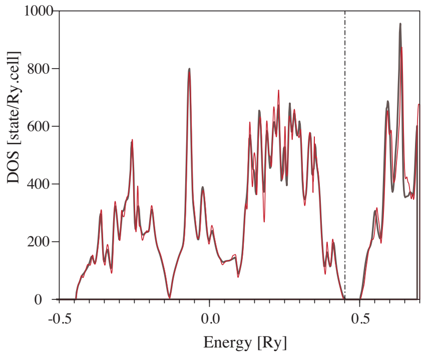


FIG. 8: DOS of $H_4$ complex (red line). DOS of bulk Si is shown a by black line. The top of occupied bands is indicated by a dashed line.

localized state which is observed in PL spectra[6]. In addition, between the $s$ and $p$ bands of the valence band, a localized state is observed at -0.12 Ry.

For $H_4$, the DOS of doped crystal is almost the same as that of bulk Si, so that the red and black lines are overlapped. The change of the electronic structure by $H_4$ can be described mostly by the rigid-band model. In this case, the role of hydrogen is a termination of a vacancy only. By considering that the concentration of the $H_4$ tetrahedron in the calculation is very high, *i.e.*, one unit per 64 atoms, it is surprising to observe that there is no consequence of the doping except perfect removing of the dangling bonds.

## S6. Charge states and the dependence on the Fermi energy

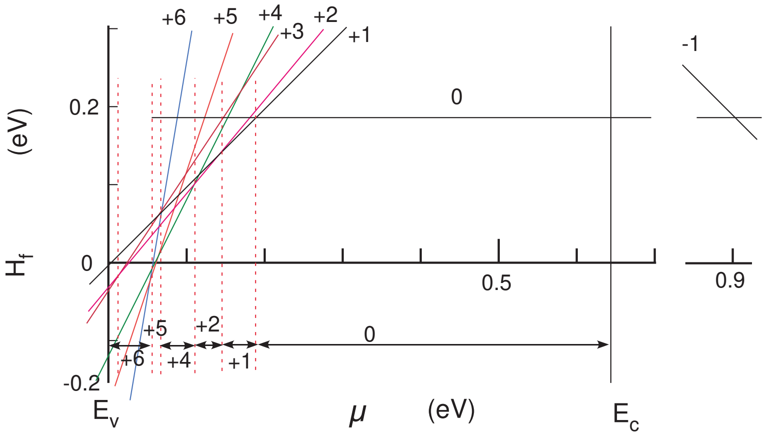


FIG. 9: Formation energy of charge states of the $Cu_4$ complex of $T$-type as a function of the Fermi level $\mu$. The top of the valence band is taken as the origin of energy.

TABLE IV: Deformation of the $Cu_4$ tetrahedron of $T$-type by changing the charge $q$. The lengths of bonds $Cu_{(s)} - Cu_{(i)}$ and $Cu_{(s)} - Si$ are listed. $D_t$ is the deviation of the bond length $Cu_{(s)} - Cu_{(i)}$ from the average length of bond $Cu_{(i)} - Cu_{(i)}$. $D_d$ is the deviation of the bond length $Cu_{(s)} - Si$ from the average length of bond $Cu_{(i)} - Si$.

| $q$ | $Cu_{(s)} - Cu_{(i)}$ (Å) | $D_t$ (%) | $Cu_{(s)} - Si$ (Å) | $D_d$ (%) |
|---|---|---|---|---|
| 0 | 2.51 | <0.1 | 2.41 | -0.7 |
| 1 | 2.56 | 3.0 | 2.45 | -2.4 |
| 2 | 2.58 | 3.6 | 2.46 | -2.8 |
| 3 | 2.60 | 2.5 | 2.47 | -2.1 |
| 4 | 2.61 | 3.2 | 2.48 | -2.5 |
| 5 | 2.65 | 3.3 | 2.50 | -2.7 |
| 6 | 2.64 | 2.1 | 2.51 | -2.2 |

Defect levels in the band gap are determined as the Fermi level at which the charge state of the defect is changed. Figure 9 shows an energy diagram of the formation energy $H_f$ of charge states of the $Cu_4$ complex of $T$-type as a function of the Fermi level $\mu$. The formation energy $H_f^q$ of charge states are calculated by

$$H_f^q = \left(E^q - E^{q-1}\right) + q\mu, \tag{1}$$

where $E^q$ is the total energy of the charge state $q$. The top of the valence band is taken as the origin of energy. In Fig. 9, the well-known underestimate of the band gap (the bottom of the conduction band $E_c = 0.64$ eV) is observed.

In the figure, we observe that all of charge states up to $q = +6$ appear in a narrow range of the band gap, which is close to the top of valence band $E_v$. When $H_f^q$ of charge states is calculated by supercells, a spurious Coulomb interaction among charged defects in different cells is known to appear. This effect becomes serious as the charge increases, because the square dependence on $q$. Various corrections for the effect have been proposed. However, it is not clear wether these methods correct the spurious Coulomb interaction or whether these overcorrect. Hence, we present the calculation without any correction. The first donor level obtained in this manner is in good agreement with the KS level. In Fig. 9, the first

donor level (0/+) is located at $E_v + 0.19$ eV. In the DOS spectrum of Fig. 7 in the main paper, the gap band appears from $E_v$ to $E_v + 0.30$ eV with the peat at $E_v + 0.11$ eV. By considering that this gap band is actually a four-fold degenerate state with a broadening of the artificial dispersion due to using supercells, the value obtained by the total-energy difference corresponds to the highest level among these four KS levels. From this result, we consider that the first donor level can be obtained by the peak position in the DOS spectrum.

Table IV shows how the $Cu_4$ tetrahedron deforms as the charge $q$ increases. For the perfect $Cu_4$ tetrahedron, of course, the notation $Cu_{(s)}$ is nonsensical. However, for the need of connectivity to $C$-type, we use the notation $Cu_{(s)}$ as one of four $Cu_{(i)}$ atoms. On positively ionizing, the $Cu_{(s)} - Cu_{(i)}$ bond is elongated by 2 to 3 %, and the tetrahedral symmetry is broken. The symmetry of all the charged states is approximately $C_{3v}$. However, because of the calculation errors, it is not certain whether this $C_{3v}$ symmetry is exact or only approximation.

---


[1] https://azuma.nims.go.jp/cms1

[2] J. P. Perdew, K. Burke, and M. Ernzerhof, Phys. Rev. Lett **78**, 1396 (1997).

[3] D. Vanderbilt, Phys. Rev. B **41**, 7892 (1990).

[4] J. C. Slater and G. F. Koster, Phys. Rev. **94**, 1498 (1954).

[5] W. A. Harrison, *Electronic Structure and the Properties of Solids: The Physics of the Chemical Bond* (W. H. Freeman and Company, San Francisco, 1980).

[6] L. Canham, G. Davies, E. C. Lightowlers, and G. W. Blackmore, Physica B **117-118**, 119 (1983).
